# Supplementary material for: HYDRA: Model Factorization Framework for Black-Box LLM Personalization
Source: arXiv:2406.02888 source file (2024-10-25)
Supplement: Supplementary file 1 [file human-eva.tex]

\subsection{Human Evaluation}
We conduct a human evaluation regarding the usefulness of retrieved items from 50 randomly sampled queries on a scale of $\{0,1,2\}$. We provide the following guidelines for three annotators to perform a rigorous human evaluation for both RAG and \method.

\begin{lstlisting}[linewidth=\columnwidth,breaklines=true,breakindent=0pt,basicstyle=\footnotesize\ttfamily]
The goal of this evaluation is to assess the usefulness of retrieved behavior records in helping or relating to specific queries in the context of target personalization tasks. Usefulness is defined by the accuracy and utility of the information in facilitating understanding or decision-making related to text classification or generation personalization tasks.
Please rate the following retrieved information with a score of 0, 1, or 2.

> 0: Useless
Definition: The information does not provide any useful insights related to the personalization task in question. It might be factually accurate but completely off-topic or not applicable to the context of target personalization tasks.

> 1: Partially Useful
Definition: The information provides some useful insights but either lacks completeness, specificity, or direct applicability to target personalization tasks. It might include behavior patterns or profile information that are relevant to the current task but do not fully support decision-making or generating content in the given context.

> 2: Very Useful
Definition: The information directly addresses the personalization task with accurate, useful, and comprehensive insights that are highly applicable to target text classification or generation tasks. It provides detailed understanding or specific examples that facilitate decision-making, understanding, or application in the given context.
\end{lstlisting}
